# Supplementary material for: Systematic Generalisation through Task Temporal Logic and Deep Reinforcement Learning
Source: arXiv:2006.08767 source file (2021-09-13)
Supplement: Supplementary file 1 [file SymbModul.tex]

% \begin{figure}
%   \centering
% \begin{minipage}{0.9\linewidth}
% \begin{algorithm}[H]
% \caption{Symbolic Module function to obtain the subtasks from the complex specification}
% \label{alg:SymbM}
% \begin{algorithmic}
% \Function{Extractor}{$\varphi$}
%     \State Initialize ordered list of sub-tasks $\mathcal{K}$
%     \State Retrieve NM's syntax $\mathcal{A}$ 
%      \State \textbf{switch} ($\varphi$) \textbf{do}
%         \State \hspace{\algorithmicindent}  \textbf{case} $\varphi \in \mathcal{A}$ \textbf{then}
        
%         \State \hspace{\algorithmicindent} \hspace{\algorithmicindent}$\mathcal{K}$.append$(T)$
%         \State \hspace{\algorithmicindent}  \textbf{case} $\varphi = T;T'$ \textbf{then}
%          \State \hspace{\algorithmicindent}  \hspace{\algorithmicindent}$\mathcal{K}$.append$({\footnotesize\textsc{Extractor}}(T))$
%             % \State 
%             \State \hspace{\algorithmicindent}  \hspace{\algorithmicindent}$\mathcal{K}$.append$({\footnotesize\textsc{Extractor}}(T'))$
            
%         \State \hspace{\algorithmicindent}  \textbf{case} $\varphi = T \cup T'$ \textbf{then}
%              \State \hspace{\algorithmicindent}  \hspace{\algorithmicindent}$t_1 \leftarrow {\footnotesize\textsc{Extractor}}(T)$
%               \State \hspace{\algorithmicindent}  \hspace{\algorithmicindent}$t_2\leftarrow {\footnotesize\textsc{Extractor}}(T')$
%              \State \hspace{\algorithmicindent} \hspace{\algorithmicindent}\textbf{if} $(t_1 \cup t_2) \in
%                         \mathcal{A}$ \textbf{then}
%              \State \hspace{\algorithmicindent}\hspace{\algorithmicindent}\hspace{\algorithmicindent}
%              $\mathcal{K}$.append$(t_1 \cup t_2)$
%               \State \hspace{\algorithmicindent} \hspace{\algorithmicindent}\textbf{else}
%                     \State \hspace{\algorithmicindent}\hspace{\algorithmicindent}\hspace{\algorithmicindent}
%              $\mathcal{K}$.append$(t_1 ;t_2)$ \\
%      \hspace{\algorithmicindent} \Return $\mathcal{K}$
% \EndFunction
% \end{algorithmic}
% \end{algorithm}
% \end{minipage}
% \end{figure}

% \begin{figure}
%   \centering
% \begin{minipage}{0.9\linewidth}
% \begin{algorithm}[H]
% \caption{Symbolic Module function to obtain the next subtask to be solved by the Neural Module}
% \label{alg:SymbM2}
% \begin{algorithmic}
% \Function{Progression}{$\mathcal{K}$, NM}
% %  \State Declare internal functions $\mathcal{L}_I$ and $R_I$
%  \State Get initial observation $z$
%  \ForAll{$\kappa \in \mathcal{K}$}
%     \Repeat
%         \State $z' \leftarrow$ $z$ extended with $\kappa$
%         \State Get new observation:  $z \leftarrow$ NM$(z')$
%         \State $p_\alpha \leftarrow \mathcal{L}_I(z)$
%         \State Reward transition: NM $\leftarrow R_I(p_\alpha)$
%         \If{$\kappa$ is $\cap$ task}
%             \State $\kappa \leftarrow p_{\alpha'}$, where $(p_{\alpha'} \neq p_\alpha) \in \kappa$
%         \EndIf
%     \Until $p_\alpha \in \kappa$
%  \EndFor
% \EndFunction
% \end{algorithmic}
% \end{algorithm}
% \end{minipage}
% \end{figure}
