# Supplementary material for: Systematic Generalisation through Task Temporal Logic and Deep Reinforcement Learning
Source: arXiv:2006.08767 source file (2021-09-13)
Supplement: Supplementary file 2 [file table7.tex]

% \begin{wraptable}{r}{6cm}
\begin{table*}
 
  \centering
  \footnotesize
  \begin{tabular}{lcccr}
\toprule
  & \multicolumn{4}{c}{TTL instruction}\\
 \cmidrule(r){2-5}
% \cmidrule(r){4-5}
% \cmidrule(r){6-7}
   & Positive & Negative & First Choice & Second Choice\\
E+MLP  &-5.95\tiny$\pm3.15$ & 
                -0.68\tiny$\pm0.33$&       
                 -2.94\tiny$\pm1.57$ 	&        
                 -3.08\tiny$\pm1.52$\\
        
E+LSTM      &-18.52\tiny$\pm0.76$ & 
                -3.10\tiny$\pm0.81$&       
                 -5.45\tiny$\pm1.89$ 	&        
                 -4.36\tiny$\pm0.32$\\
                 
2-Layer CNN   &-1.46\tiny$\pm2.74$ & 
                0.68\tiny$\pm0.19$&       
                 0.15\tiny$\pm0.88$ 	&        
                 0.26\tiny$\pm0.38$\\
ResNet   &0.33\tiny$\pm0.69$ & 
                0.65 \tiny$\pm0.54$&       
                 0.9 \tiny$\pm0.19$ 	&        
                 0.82\tiny$\pm0.22$\\

 \bottomrule
\end{tabular}
 \caption{Average reward obtained in the 500 binary choice maps with deceptive instructions. Here lower is better.}
   \label{table:BCDFake}
\end{table*}
% \end{wraptable}
