# Supplementary material for: Systematic Generalisation through Task Temporal Logic and Deep Reinforcement Learning
Source: arXiv:2006.08767 source file (2021-09-13)
Supplement: Supplementary file 3 [file table9.tex]

% \begin{wraptable}{r}{6cm}
\begin{table*}[t]
  \centering
  \footnotesize
\begin{tabular}{lcccccr}
\toprule
  & \multicolumn{3}{c}{Positive} &  \multicolumn{3}{c}{Negative} \\
 \cmidrule(r){2-4}
\cmidrule(r){5-7}
  Difference &E+MLP&RE+MLP&E+LSTM&E+MLP&RE+MLP&E+LSTM \\
\midrule
  $\sim 35 \%$  & 1.00 &1.00  &	1.00 & 1.00&   
        1.00  &	1.00\\
 $\sim 20 \%$  & 0.73\tiny$\pm0.04$ &0.99\tiny$\pm0.02$  &	0.89\tiny$\pm0.05$ & 
        0.37\tiny$\pm0.11$  &   
        0.81\tiny$\pm0.01$   &	0.60\tiny$\pm0.25$ \\
$\sim 15 \%$  & 0.71\tiny$\pm0.04$ &0.95\tiny$\pm0.02$  &	0.78\tiny$\pm0.06$ & 
        0.57\tiny$\pm0.11$  &   
        0.79\tiny$\pm0.00$   &	0.15\tiny$\pm0.32$ \\
$\sim 9 \%$  & 0.58\tiny$\pm0.05$ &0.93\tiny$\pm0.03$  &	0.86\tiny$\pm0.04$ & 
        0.78\tiny$\pm0.17$  &   
        0.65\tiny$\pm0.04$   &	0.43\tiny$\pm0.33$ \\
$ <2 \%$  & 0.13\tiny$\pm0.14$ &0.23\tiny$\pm0.07$  &	0.45\tiny$\pm0.05$ & 
        0.29\tiny$\pm0.12$  &   
        0.10\tiny$\pm0.09$   &	0.09\tiny$\pm0.28$ \\

\bottomrule
\end{tabular}
\caption{Performance in the BCMs given the similarity of two objects, $|\mathcal{X}_{1}|=10$}
   \label{table:similarity}
\end{table*}
% \end{wraptable}
